# Supplementary material for: NukesFormers: Unpaired Hyperspectral Image Generation with Non-Uniform Domain Alignment
Source: arXiv:2503.07004 source file (2025-03-10)
Supplement: Supplementary file 1 [file X_suppl.tex]

\clearpage
\setcounter{page}{1}
\maketitlesupplementary

\section{Introduction of Supplementary Material}
\label{sec:rationale}
Owing to the space constraints in the main body of the paper, a Supplementary Material has been prepared to provide supplementary information regarding relevant parameter calculations, experimental analyses, and result visualizations. Specifically, the Supplementary Material is structured into the following three principal sections:
\begin{itemize}
\item Detailed calculations of the relevant parameter indicators;
\item In-depth details of the experimental design and a comprehensive description of the specific datasets used; 
\item Visualizations of the comparison and ablation experiments.
\end{itemize}

\section{Details of Relevant Parameter}
In this section, we provide the mathematical formulas for three evaluation criteria used in our paper about the hyperspectral image generation (HIG). The detailed mathematical calculation formulas for root mean square error (RMSE), mean relative absolute error (MRAE), peak signal-to-noise ratio (PSNR) and spectral angle mapper (SAM), are shown below.

\begin{equation}
\label{deqn_ex_param1}
RMSE=\sqrt{\frac{1}{N}\sum_{n=1}^N(\textbf{X}[n]-\textbf{X}_{rec}[n])^{2}}
\end{equation}

\begin{equation}
\label{deqn_ex_param2}
MRAE= \frac{1}{N}\sum_{n=1}^N\frac{|\textbf{X}[n]-\textbf{X}_{rec}[n]|}{\textbf{X}[n]}
\end{equation}

\begin{equation}
\label{deqn_ex_param3}
PSNR=10lg\left(\frac{(2^{8}-1)^{2}}{MSE(\zeta(\textbf{X}), \zeta(\textbf{X}_{rec}))}\right)
\end{equation}

\begin{equation}
\label{deqn_ex_param5}
SSIM=\frac{(2\mu_X\mu_{X_{rec}} + c_1)(2\sigma_{XX_{rec}} + c_2)}{(\mu_X^2 + \mu_{X_{rec}}^2 + c_1)(\sigma_X^2 + \sigma_{X_{rec}}^2 + c_2)}
\end{equation}

\begin{equation}
\label{deqn_ex_param4}
    SAM = \frac{1}{N} \sum_{bi=1}^{N}\left(\frac{180}{\pi} \arccos \frac{\left\langle \mathbf{X}[bi], \mathbf{X}_{rec}[bi] \right\rangle}{\left\|\mathbf{X}[bi] \right\|_2\left\|\mathbf{X}_{rec}[bi]\right\|_2}\right)
\end{equation}

in which the $N$ represents the number of bands, $\textbf{X}[n]$ and $\textbf{X}_{rec}[n]$ stand for the n-th band in real HSI $\textbf{X}$ and the n-th band in recovery HSI $\textbf{X}_{rec}$ respectively and $\zeta(\textbf{X})$ is the the operation of enlarging $\textbf{X}$ to (0, 255). And the mean-square error (MSE) is defined by $MSE(\textbf{u}, \textbf{v})=\frac{1}{D}\sum^{D}_{d=1}(\textbf{u}_{d}-\textbf{v}_{d})^{2}$, in which $D$ stands for the number of pixel. In addition, $\mu$ denotes the mean value of the corresponding parameter, $\sigma$ represents the covariance of the corresponding parameter, and c  is set as the minimum value, which serves to prevent the need for zero supplementation.
\begin{figure*}[!t]
\centering
\includegraphics[width=0.95\linewidth]{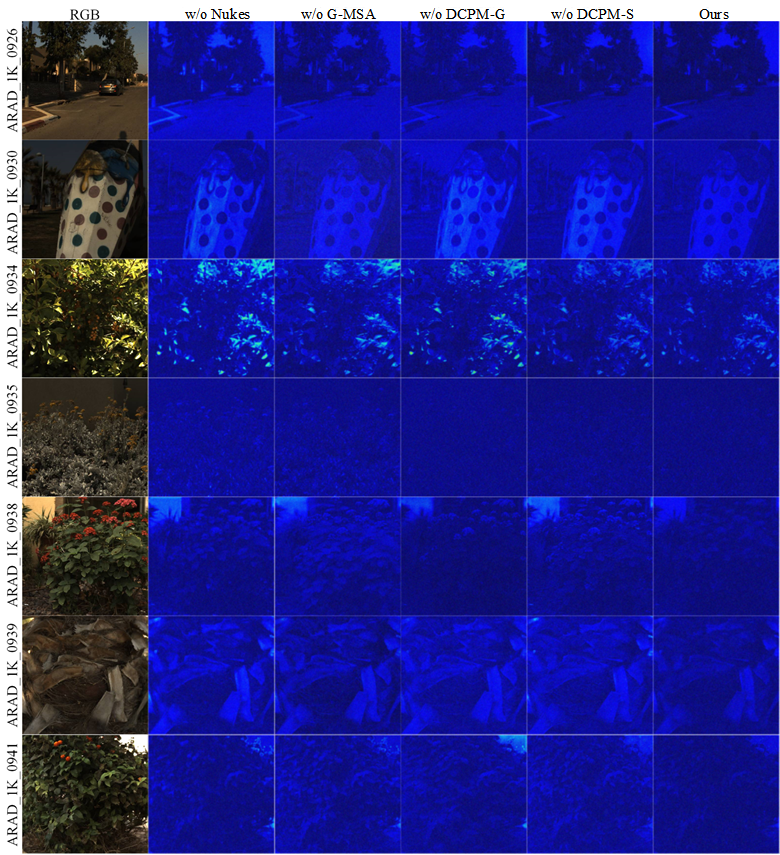}
\caption{\textbf{Visual Comparison Results}. Line 1-7: the RMSE error map of seven distinct validation images in NTIRE 2022. Column 1: The RGB images of seven different scenes. Column 2-5: The corresponding RMSE error map lacking a key block. Column 6: The RMSE error map of NukesFormers.}
\label{image4}
\end{figure*}

Specifically, the RMSE and MRAE are used to calculate the pixel-wise disparity between ground truth and recovery HSIs. And the PSNR is one of the indexes to measure the quality of $\textbf{X}_{rec}$. Furthermore, the structural similarity (SSIM) of each band is employed to measure the similarity of each band between ground truth and recovery HSIs. The smaller RMSE, MRAE, and larger PSNR and SSIM indicate better HIG performance in different views respectively.
\section{Experiments Setting}
In comparison experiments, we select three benchmark dataset, consisting of NTIRE 2020 Clean Track \cite{arad2020ntire}, NTIRE 2022 \cite{arad2022ntire} and CAVE \cite{yasuma2010generalized}. In NTIRE 2020 Clean Track dataset, there are 450 paired RGB-HSIs and we partition them into two non-overlapping sets of 225 RGB images and 225 HSIs, respectively, which are used to construct the UnHIG experiment. We also adopt the standard validation set consisting of 10 pairs of images. Additionally, all images share the same spatial resolution of $512\times482$ and 31 bands spanning the 400-700 nm range. Similar to NTIRE 2020, the NTIRE 2022 dataset has the same spatial and spectral resolution as the former. A corpus of 900 pairs of images in the training set and an additional 50 pairs in the validation set are utilized in experiments. The CAVE is a slim dataset for hyperspectral images (HSIs) tasks, including 32 512x512 HSIs with 31 bands (400-700 nm), in which the 24 patches are selected randomly for training and the rest of them are prepared to validate.

\begin{figure*}[!t]
\centering
\includegraphics[width=0.95\linewidth]{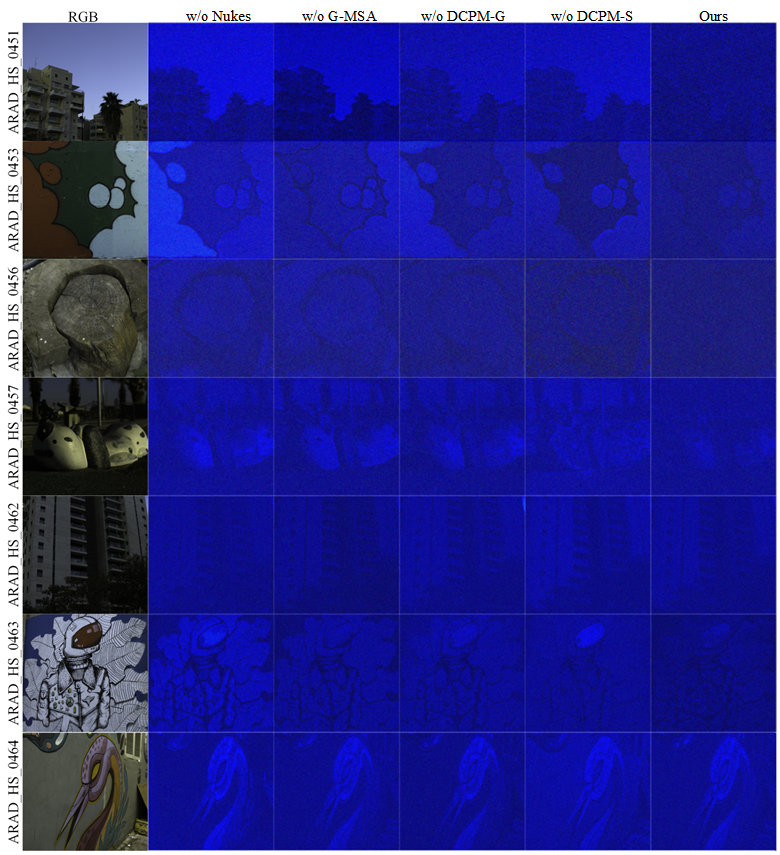}
\caption{\textbf{Visual Comparison Results}. Line 1-7: the RMSE error map of seven distinct validation images in NTIRE 2020 Clean Track. Column 1: The RGB images of seven different scenes. Column 2-5: The corresponding RMSE error map lacking a key block. Column 6: The RMSE error map of NukesFormer.}
\label{image5}
\end{figure*}
Furthermore, to demonstrate the efficiency and adaptability of our proposed framework, we integrate HSCNN+ \cite{shi2018hscnn+}, HRNet \cite{zhao2020hierarchical}, HDNet \cite{hu2022hdnet}, AWAN \cite{li2020adaptive}, Restormer\cite{zamir2022restormer}, and MST++ \cite{cai2022mst++} as feature extraction units using existing state-of-the-art methods. As the winner network of the NTIRE 2018 competition, HSCNN+ employs two DCNN modules to achieve exceptional image reconstruction results. Similarly, the convolutional residual module integrated into the HRNet architecture extracts deep-level image information and secured victory in the NTIRE 2020 Realworld Track championship. AWAN, on the other hand, utilizes a stacked attention mechanism that enhances feature connections between channels, leading to improved reconstruction performance. HDNet exploits the spatial-spectral domain learning to reconstruct the duel domain information, while fusing the group and input feature. Furthermore, recent advances in transformer-based HIG networks have demonstrated significant progress. Restormer, for instance, focuses on long-range pixel interactions, yielding notable results for large image reconstructions. As one of the most anticipated HIG methods, MST++ expertly employs a multilayer Transformer framework and emerged as the champion of the NTIRE 2022 competition. Then, the existing unpaired framework UnGUN \cite{qu2023unmixing} is introduced as the direct competitive method.

Obviously, the reconstructed HSIs exhibit a global distortion and local texture degradation in the error maps as shown in Fig.\ref{image4}, attributable to the absence of high-frequency components after removal by the Nukes. Additionally, the significance of aligning the null space through the DCPM method is also demonstrated in the aforementioned experiments. Compared to the w/o DCPM, the proposed NukesFormers shows a significantly dark appearance in error maps.
\section{Visual Performance of Ablation Study}
The visual performance about the ablation experiments of key modules is shown in the session.
\label{sec:visual}

In addition, we also carry the ablation study in NTIRE 2020 Clean Track. The visiable results have been shown in Fig.\ref{image5}, which implies the importance of mining high-frequency components in range space and aligning the null space with unpaired images in the UnHIG.
